# Supplementary material for: SPnet: Estimating Garment Sewing Patterns from a Single Image
Source: arXiv:2312.16264 source file (2023-12-26)
Supplement: Supplementary file 1 [file Appendix.tex]

\documentclass[../eg2024main.tex]{subfiles}
\begin{document}
\appendix
\section{Network architecture}
\begin{figure}[t]
  \centering
  \includegraphics[width=.9\linewidth]{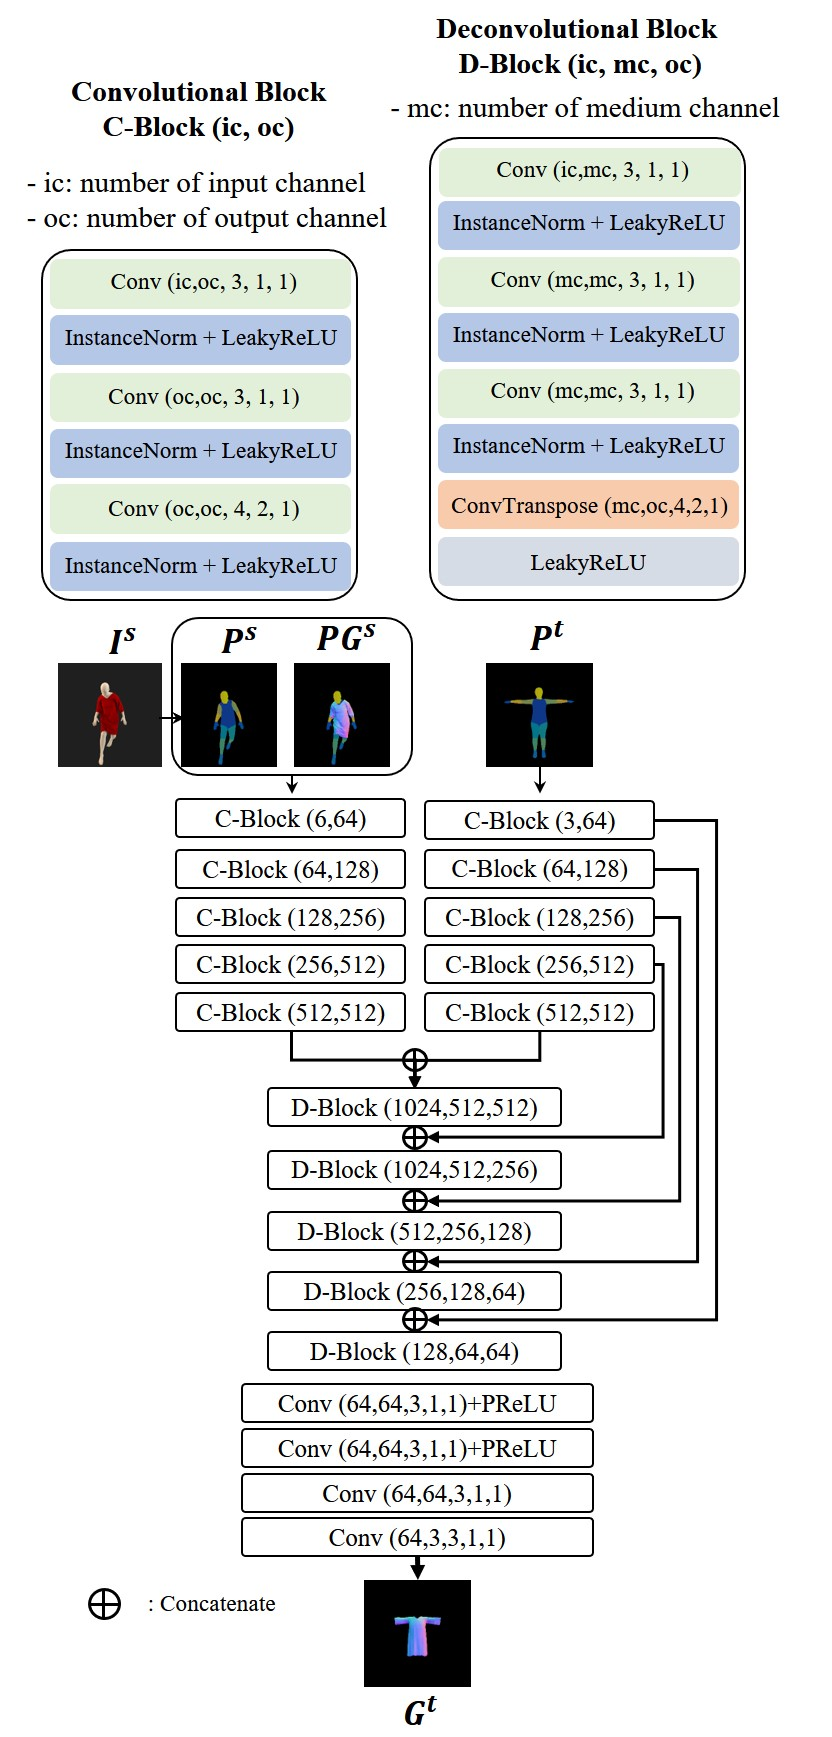}
  \caption{The detailed structure of T-pose garment predictor. The architecture primarily consists of Convolutional Blocks (C-Block) and Deconvolutional Blocks (D-Block), with a LeakyReLU coefficient uniformly set at 0.2.}
  \label{fig:appendix1}
\end{figure}
\begin{figure}[t]
  \centering
  \includegraphics[width=.9\linewidth]{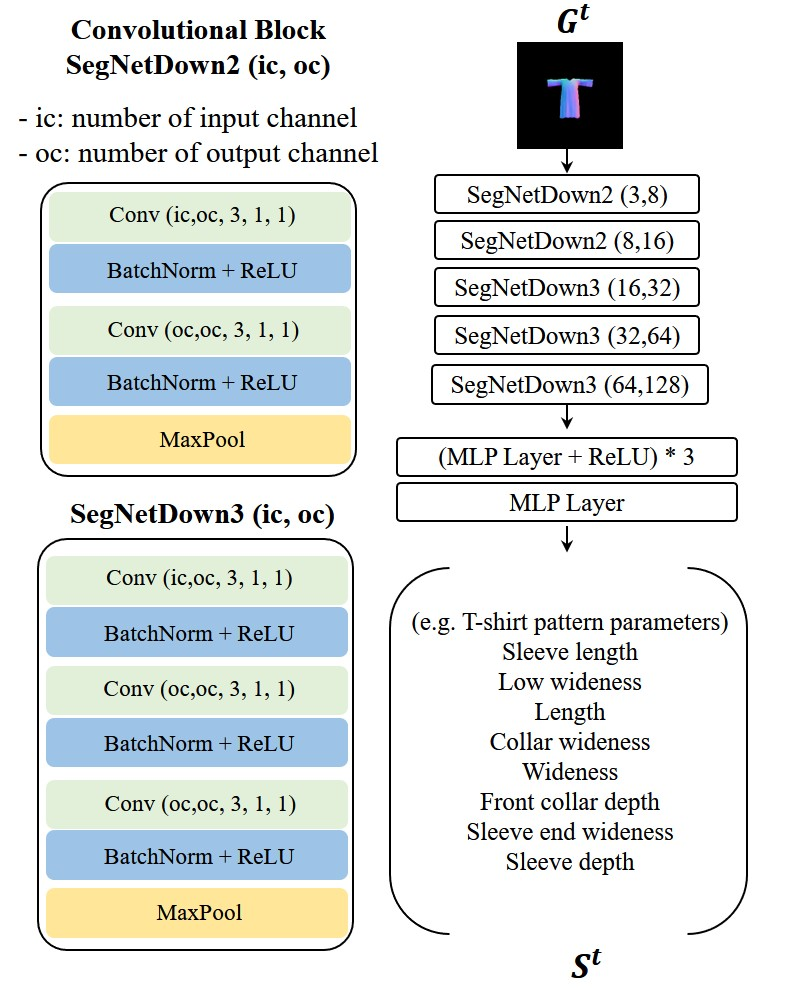}
  \caption{The detailed structure of the sewing pattern parameter predictor.}
  \label{fig:appendix2}
\end{figure}

Figure \ref{fig:appendix1} depicts the detailed architecture of the T-pose garment predictor. This architecture is inspired by the "SilNet" model from \cite{yoon2021pose}. Instead of predicting the combined silhouette of body and clothing at the target pose as they did, we focus on predicting the T-pose garment image \textit{$G^t$}. The information obtained from concatenating the \textit{$P^s$} and \textit{$PG^s$} of Image \textit{$I^s$} is passed through the C-Block, and the same process applies to the \textit{$P^t$} image. As the information from these two C-Blocks
integrates and passes through the D-Block, information about the T-pose is conveyed through a skip connection approach, thereby assisting the learning of clothing in T-pose.

Figure \ref{fig:appendix2} presents  the detailed architecture of the sewing pattern parameter predictor. To predict the parameters \textit{$S^t$}, which consist of fewer than 10 parameters from high-dimensional images, a lighter feature that can effectively encapsulate image information is required. We initially train a SegNet\cite{badrinarayanan2017segnet}, an encoder-decoder architecture composed of convolutional layers. Subsequently, employing the learned filters, we decrease the dimension of \textit{$G^t$} via SegNetDown blocks (2,3). Finally, we can predict the sewing pattern parameters \textit{$S^t$} through a Multilayer Perceptron (MLP) process.

% \begin{figure}[t]
%   \centering
%   \includegraphics[width=.9\linewidth]{appendix_1_final.jpg}
%   \caption{The detailed structure of T-pose garment predictor. The architecture primarily consists of Convolutional Blocks (C-Block) and Deconvolutional Blocks (D-Block), with a LeakyReLU coefficient uniformly set at 0.2.}
%   \label{fig:appendix1}
% \end{figure}
% \begin{figure}[t]
%   \centering
%   \includegraphics[width=.9\linewidth]{appendix_2_final.jpg}
%   \caption{The detailed structure of the sewing pattern parameter predictor.}
%   \label{fig:appendix2}
% \end{figure}

\end{document}
